# Supplementary material for: Responses to COVID-19 with Probabilistic Programming
Source: arXiv:2106.00192 source file (2021-06-01)
Supplement: Supplementary file 2 [file appendix_simulation.tex]

\begin{table}[h]
\centering
\caption{Loss regarding to applied policies. The most effective policy combination is listed at the top. The meaning of policy notation is as follows. None: Doing nothing, Uppercase: full efficacy, lower case: half efficacy, L/l: \textbf{L}ockdown, T/t:  \textbf{T}racing with distancing, D/d: \textbf{D}istancing, M: \textbf{M}asks and hygiene.
\textit{Example: L $\rightarrow$ l $\rightarrow$ D denotes the consecutive policy execution of full lockdown (1st month), half lockdown (2nd month) and full distancing (3rd month)}.
}
\small

% text should be left-aligned, numbers should be right aligned
\begin{tabular}{lrrr}

\toprule
\textbf{Policy Combination} & \textbf{Total Cases}                & \textbf{Total Deaths}              & \textbf{Total Loss (Billion \$)}        \\ \midrule
{\color[HTML]{000000} \textbf{T $\rightarrow$ T $\rightarrow$ None }}                                  & {\color[HTML]{000000} 11,749}  & {\color[HTML]{000000} 218}   & {\color[HTML]{000000} 2.097}   \\
{\color[HTML]{000000} \textbf{mT $\rightarrow$ T $\rightarrow$ None }}                                 & {\color[HTML]{000000} 11,509}  & {\color[HTML]{000000} 215}   & {\color[HTML]{000000} 2.136}   \\
{\color[HTML]{000000} \textbf{T $\rightarrow$ T $\rightarrow$ m}}                                  & {\color[HTML]{000000} 11,381}  & {\color[HTML]{000000} 218}   & {\color[HTML]{000000} 2.155}   \\
{\color[HTML]{000000} \textbf{T $\rightarrow$ mT $\rightarrow$ None }}                                 & {\color[HTML]{000000} 11,694}  & {\color[HTML]{000000} 218}   & {\color[HTML]{000000} 2.156}   \\
{\color[HTML]{000000} \textbf{dT $\rightarrow$ T $\rightarrow$ None }}                                 & {\color[HTML]{000000} 11,237}  & {\color[HTML]{000000} 212}   & {\color[HTML]{000000} 2.176}   \\
{\color[HTML]{000000} \textbf{MT $\rightarrow$ T $\rightarrow$ None }}                                 & {\color[HTML]{000000} 11,277}  & {\color[HTML]{000000} 212}   & {\color[HTML]{000000} 2.176}   \\
{\color[HTML]{000000} \textbf{mT $\rightarrow$ T $\rightarrow$ m}}                                 & {\color[HTML]{000000} 11,167}  & {\color[HTML]{000000} 215}   & {\color[HTML]{000000} 2.194}   \\
{\color[HTML]{000000} \textbf{mT $\rightarrow$ mT $\rightarrow$ None }}                                & {\color[HTML]{000000} 11,457}  & {\color[HTML]{000000} 215}   & {\color[HTML]{000000} 2.196}   \\
{\color[HTML]{000000} \textbf{mdT $\rightarrow$ T $\rightarrow$ None }}                                & {\color[HTML]{000000} 11,096}  & {\color[HTML]{000000} 210}   & {\color[HTML]{000000} 2.224}   \\
{\color[HTML]{000000} \textbf{DT $\rightarrow$ T $\rightarrow$ None }}                                 & {\color[HTML]{000000} 10,764}  & {\color[HTML]{000000} 207}   & {\color[HTML]{000000} 2.259}   \\
\multicolumn{4}{c}{{\color[HTML]{000000} \textbf{...}}}                                                                                                                       \\
{\color[HTML]{000000} \textbf{T $\rightarrow$ T $\rightarrow$ T}}                                  & {\color[HTML]{000000} 11,068}  & {\color[HTML]{000000} 217}   & {\color[HTML]{000000} 2.339}   \\
{\color[HTML]{000000} \textbf{L $\rightarrow$ L $\rightarrow$ L}}                                  & {\color[HTML]{000000} 11,068}  & {\color[HTML]{000000} 217}   & {\color[HTML]{000000} 3.060}   \\
{\color[HTML]{000000} \textbf{D $\rightarrow$ D $\rightarrow$ D}}                                  & {\color[HTML]{000000} 26,020}  & {\color[HTML]{000000} 437}   & {\color[HTML]{000000} 3.931}   \\
{\color[HTML]{000000} \textbf{M $\rightarrow$ M $\rightarrow$ M}}                                  & {\color[HTML]{000000} 597,562} & {\color[HTML]{000000} 38,523} & {\color[HTML]{000000} 272.798} \\
\multicolumn{4}{c}{{\color[HTML]{000000} \textbf{...}}}                                                                                                                       \\
{\color[HTML]{000000} \textbf{ None  $\rightarrow$ m $\rightarrow$ None }}                                  & {\color[HTML]{000000} 857,544} & {\color[HTML]{000000} 62,651} & {\color[HTML]{000000} 443.003} \\
{\color[HTML]{000000} \textbf{ None  $\rightarrow$ None  $\rightarrow$ d}}                                  & {\color[HTML]{000000} 884,114} & {\color[HTML]{000000} 65,385} & {\color[HTML]{000000} 462.388} \\
{\color[HTML]{000000} \textbf{ None  $\rightarrow$ None  $\rightarrow$ M}}                                  & {\color[HTML]{000000} 885,390} & {\color[HTML]{000000} 65,467} & {\color[HTML]{000000} 462.964} \\
{\color[HTML]{000000} \textbf{ None  $\rightarrow$ None  $\rightarrow$ m}}                                  & {\color[HTML]{000000} 892,702} & {\color[HTML]{000000} 65,935} & {\color[HTML]{000000} 466.212} \\
{\color[HTML]{000000} \textbf{ None  $\rightarrow$ None  $\rightarrow$ None}}                                  & {\color[HTML]{000000} 900,090} & {\color[HTML]{000000} 66,406} & {\color[HTML]{000000} 469.480} \\ 
\bottomrule
\end{tabular}
\label{tab:simulation_result}
\end{table}
